# Supplementary material for: Effectiveness of Adversarial Examples and Defenses for Malware Classification
Source: arXiv:1909.04778 source file (2019-09-10)
Supplement: Supplementary file 1 [file appendix.tex]

\section*{Appendix}

\subsection*{Attacks}
\subsubsection*{Feature enabling and disabling}
\begin{table}[H]
	\centering
	\begin{tabular}{|m{1cm}|c|c|c|c|c|c|} 
		\hline
		Attack						& acc & acc adv & FNR  & FNR adv  & change & evasion\\ [0.5ex] 
		\hline
		\hline
		dec\_pos					& 0.93 & 0.62   & 0.12 & 0.56     & 6.25  & 1.0 \\ 
		\hline
		inc\_neg 					& 0.93 & 0.62   & 0.12 & 0.56     & 13.57 & 1.0 \\ 
		\hline
		dec\_pos and inc\_neg		& 0.93 & 0.62   & 0.12 & 0.56     & 1.37  & 1.0 \\
		\hline
		rand. dec\_pos				& 0.93 & 0.62   & 0.12 & 0.56     & 7.17  & 1.0 \\
		\hline
		rand. inc\_neg      		& 0.93 & 0.93   & 0.12 & 0.12     & 0.57  & 0.12 \\
		\hline
		rand dec\_pos and inc\_neg	& 0.93 & 0.63  & 0.12  & 0.54     & 0.0  & 0.96 \\		
		\hline
	\end{tabular}
	\label{appendix:attacks_dec_pos_inc_neg}
	\caption{Stokes et. al \cite{DBLP:journals/corr/abs-1712-05919} approaches based on enabling and disabling features based on their Jacobian. Numbers reported on APDS }
\end{table}

\red{PUT MALINE DATA HERE}

\subsubsection*{$FGSM^k$}
\begin{table}[H]
	\centering
	\begin{tabular}{|c|c|c|c|c|c|c|} 
		\hline
		Attack		& acc & acc adv & FNR  & FNR adv  & change & evasion\\ [0.5ex] 
		\hline
		\hline
		$dFGSM^k$	& 0.93 & 0.62   & 0.12 & 0.56     & 70.64  & 1.0 \\ 
		\hline
		$rFGSM^k$ 	& 0.93 & 0.62   & 0.12 & 0.56     & 70.64  & 1.0 \\ 
		\hline
		$BGA^k$		& 0.93 & 0.91   & 0.12 & 0.12     & 24.50  & 0.12 \\
		\hline
		$BCA^k$		& 0.93 & 0.90   & 0.12 & 0.12     & 2.14 & 0.14 \\
		\hline
	\end{tabular}
	\caption{Al-Dujaili et. al \cite{DBLP:journals/corr/abs-1801-02950} iterative $FGSM^k$ based approaches with random $rFGSM^k$ and deterministic rounding $dFGSM^k$. As well as bit gradient ascent $BGA^k$ and bit coordinate ascent $BCA^k$. Numbers reported on $\text{Drebin}_{500} $ }
	\label{attacks_fgsm_and_bit_ascent}
\end{table}

\subsection*{Defenses}
\subsubsection*{Distillation}
\begin{table}[H]
	\centering
	\begin{tabular}{lrr}
		\toprule
		Attack  						& undefended	& defended	\\
		\midrule
		natural                     	& 5.6			& 100.0	\\
		dfgsm\_k                    	& 15.0			& 100.0 \\
		rfgsm\_k                    	& 15.0			& 100.0 \\
		bga\_k                      	& 5.6			& 100.0	\\
		bca\_k                   		& 12.7			& 100.0	\\
		JSMA                        	& 32.8			& 100.0 \\
		random\_inc\_neg            	& 6.0			& 100.0	\\
		dec\_pos                    	& 25.4			& 100.0	\\
		inc\_neg                    	& 32.8			& 100.0	\\
		random\_dec\_pos            	& 24.7			& 100.0 \\
		random\_dec\_pos\_inc\_neg  	& 18.1			& 100.0	\\
		dec\_pos\_inc\_neg          	& 27.0			& 100.0	\\
		malgan                      	& 0.0			& 100.0	\\
		\bottomrule
	\end{tabular}
	\caption{Evasion rates in \% of various attacks on the undefended and defended with Distillation at temperature 10. Models are trained on \Drebinfive }
\end{table}
	
\subsubsection*{Random Feature Nullification}
\begin{table}[H]
	\centering
	\begin{tabular}{lrr}
		\toprule
		Attack  						& undefended	& defended	\\
		\midrule
		natural                     	& 5.6			& 22.0	\\
		dfgsm\_k                    	& 15.0			& 19.6 \\
		rfgsm\_k                    	& 15.0			& 17.5	\\
		bga\_k                      	& 5.6			& 24.5	\\
		bca\_k                   		& 12.7			& 36.9	\\
		JSMA                        	& 32.8			& 67.8 \\
		random\_inc\_neg            	& 6.0			& 100.0	\\
		dec\_pos                    	& 25.4			& 90.5	\\
		inc\_neg                    	& 32.8			& 60.7	\\
		random\_dec\_pos            	& 24.7			& 70.4 \\
		random\_dec\_pos\_inc\_neg  	& 18.1			& 17.8	\\
		dec\_pos\_inc\_neg          	& 27.0			& 88.3	\\
		malgan                      	& 0.0			& 89.9	\\
		\bottomrule
	\end{tabular}
	\caption{Evasion rates in \% of various attacks on the undefended and defended with Distillation at temperature 10. Models are trained on \Drebinfive }
\end{table}
